# Supplementary material for: Evolving GAN Formulations for Higher Quality Image Synthesis
Source: arXiv:2102.08578 source file (2021-10-28)
Supplement: Supplementary file 1 [file appendix.tex]

\appendix

%\section{Broader Impact}
%This paper presents TaylorGLO, a new technique for automatically discovering new, more optimal loss functions for neural networks. Models trained with TaylorGLO loss functions achieve higher accuracies and are more robust. These properties allow TaylorGLO to be used as a general technique that can help humans building machine learning systems to train better models with their finite efforts.

%TaylorGLO uses a population-based search to optimize loss functions that can require many models to be trained. This methodology requires a large amount of compute power that scales with the time needed to train individual models. In addition to requiring greater amounts of electricity, these high compute costs can put this technique out of reach of those who do not have access to such resources. TaylorGLO attempts to ameliorate this with a parameter that can tune a trade-off between computation and loss function performance estimate accuracy.

\section{Experimental setup}
\label{ap:setup}

The following subsections cover specific experimental setup details. The three evaluated datasets are detailed in how they were used, along with implementation details.

\subsection{MNIST}

The first domain was MNIST Handwritten Digits, a widely used dataset where the goal is to classify $28\times28$ pixel images as one of ten digits. MNIST has 55,000 training samples, 5,000 validation samples, and 10,000 testing samples. The dataset is well understood and relatively quick to train, and forms a good foundation for understanding how TaylorGLO evolves loss functions.

The basic CNN architecture evaluated in the GLO study \citep{gonzalez2019glo} can also be used to provide a direct point of comparison with prior work on MNIST. Importantly, this architecture includes a dropout layer \citep{hinton2012improving} for explicit regularization. As in GLO, training is based on stochastic gradient descent (SGD) with a batch size of 100, a learning rate of 0.01, and, unless otherwise specified, occurred over 20,000 steps.

\subsection{CIFAR-10 and CIFAR-100}

To validate TaylorGLO in a more challenging context, the CIFAR-10 \citep{krizhevsky2009learning} dataset was used. It consists of small $32\times32$ pixel color photographs of objects in ten classes. CIFAR-10 traditionally consists of 50,000 training samples, and 10,000 testing samples; however 5,000 samples from the training dataset were used for validation of candidates, resulting in 45,000 training samples.

Models were trained with their respective hyperparameters from the literature. Inputs were normalized by subtracting their mean pixel value and dividing by their pixel standard deviation. Standard data augmentation techniques consisting of random horizontal flips and croppings with two pixel padding were applied during training.

CIFAR-100 is a similar, though significantly more challenging, dataset where a different set of 60,000 images is divided into 100 classes, instead of 10. The same splits for training, validation, and testing were used for CIFAR-100 as for CIFAR-10, and evaluate TaylorGLO further.

\subsection{SVHN}

The Street View House Numbers \citep[SVHN;][]{svhn} dataset is another image classification domain that was used to evaluate TaylorGLO, consisting of $32\times32$ pixel images of numerical digits from Google Street View. SVHN consists of 73,257 training samples, 26,032 testing samples, and 531,131 supplementary, easier training samples. To reduce computation costs, supplementary examples were not used during training; this fact explains why presented baselines may be lower than other SVHN baselines in the literature. Since a validation set is not in the standard splits, 26,032 samples from the training dataset were used for validation of candidates, resulting in 47,225 training samples.

As with CIFAR-10, models were trained with their respective hyperparameters from the literature and with the same data augmentation pipeline.

\subsection{Candidate evaluation details}

During candidate evaluation, models were trained for 10\% of a full training run on MNIST, equal to 2,000 steps (i.e., four epochs). An in-depth analysis on the technique's sensitivity to training steps during candidate evaluation is provided in Appendix~\ref{ap:sensitivity}---overall, the technique is robust even with few training steps. However, on more complex models with abrupt learning rate decay schedules, greater numbers of steps provide better fitness estimates.

\subsection{Statistical testing}

Statistical significance tests define a null hypothesis and reject it if a $p$-value is below a predefined significance level, typically $0.05$. A $p$-value is the probability of obtaining extreme results at the same level or greater than the results observed given that the null hypothesis is true.

When comparing results in this paper, a one-tailed null hypothesis is typically used:
\begin{equation}
H_0: \neg \left( \mu_1 < \mu_2 \right) ,
\end{equation}
where $\mu_1$ and $\mu_2$ are mean values from two separate sets of training sessions. The rejection of this null hypothesis implies that $\mu_2$ is statistically significantly larger than $\mu_1$. Thus, the change between the two sets of training sessions is robust to training stochasticity, such as from varying weight initializations.

Throughout this paper, Welch's $t$-Test \cite{welch1947ttest} is used to determine statistical significance when comparing sets of results which may not have equal variances. It is also a better fit than Student's $t$-Test due to its higher robustness and statistical power \cite{ruxton2006unequal}.

\subsection{Implementation details}

Due to the number of partial training sessions that are
needed to evaluate TaylorGLO loss function candidates, training
was distributed across the network to a cluster, composed of dedicated machines with NVIDIA GeForce GTX 1080Ti GPUs. Training itself was implemented with
TensorFlow \citep{tensorflow} in Python. The primary components of TaylorGLO
(i.e., the genetic algorithm and CMA-ES) were implemented in the
Swift programming language which allows for easy parallelization. These components run centrally on one machine and
asynchronously dispatch work to the cluster. %The implementation made use of the open-source SwiftCMA \citep{swiftcma} library for CMA-ES.

Training for each candidate was aborted and retried up to two additional times if validation accuracy was below 0.15 at the tenth epoch. This method helped reduce computation costs.

\section{Illustrating the evolutionary process}
\label{ap:process}

\begin{figure}
  \centering
  \includegraphics[width=0.9\linewidth]{images/mnist_tsne.pdf}
  \caption{A visualization of all TaylorGLO loss function candidates using t-SNE \citep{tsne} on MNIST. Colors map to each candidate's generation. Loss function populations show an evolutionary path and focus over time towards functions that perform well, consistent with the convergence and settling in Figure~\ref{fig:mnist_lossfns}.}
  \label{fig:mnist_tsne}
  \vspace{-1em}
\end{figure}

The TaylorGLO search process can be illustrated with t-SNE dimensionality reduction \citep{tsne} on \emph{every} candidate loss function within a run (Figure~\ref{fig:mnist_tsne}).  The initial points (i.e.\ loss functions) are initially widespread on the left side, but quickly migrate and spread to the right as CMA-ES explores the parameter space, and eventually concentrate in a smaller region of dark red points. This pattern is consistent with the convergence and settling in Figure~\ref{fig:mnist_lossfns}.

\section{Top MNIST loss function}

The best loss function obtained from running TaylorGLO on MNIST was found in generation 74. This function, with parameters $\vec{\theta} = \langle 11.9039$, $-4.0240$, $6.9796$, $8.5834$, $-1.6677$, $11.6064$, $12.6684$, $-3.4674 \rangle$ (rounded to four decimal-places), achieved a 2k-step validation accuracy of 0.9950 on its single evaluation, higher than 0.9903 for the cross entropy loss. This loss function was a modest improvement over the previous best loss function from generation 16, which had a validation accuracy of 0.9958.
%6.9795621992583108,8.5833826548675312,-1.6676703023074477,11.606376507890865,12.66843455324307,-3.4674186166093821,11.903859924068879,-4.0239925257451645

\section{MNIST evaluation length sensitivity}
\label{ap:sensitivity}

\paragraph{200-step} TaylorGLO is surprisingly resilient when evaluations during evolution are shortened to 200 steps (i.e., 0.4 epochs) of training. With so little training, returned accuracies are noisy and dependent on each individual network's particular random initialization. On a 60-generation run with 200-step evaluations, the best evolved loss function had a mean testing accuracy of 0.9946 across ten samples, with a standard deviation of 0.0016. While slightly lower, and significantly more variable, than the accuracy for the best loss function that was found on the main 2,000-step run, the accuracy is still significantly higher than that of the cross-entropy baseline, with a $p$-value of $6.3\e{-6}$. This loss function was discovered in generation 31, requiring 1,388.8 2,000-step-equivalent partial evaluations. That is, evolution with 200-step partial evaluations is over three-times less sample efficient than evolution with 2,000-step partial evaluations.

\paragraph{20,000-step} On the other extreme, where evaluations consist of the same number of steps as a full training session, one would expect better loss functions to be discovered, and more reliably, because the fitness estimates are less noisy. Surprisingly, that is not the case: The best loss function had a mean testing accuracy of 0.9945 across ten samples, with a standard deviation of 0.0015. While also slightly lower, and also significantly more variable, than the accuracy for the best loss function that was found on the main 2,000-step run, the accuracy is significantly higher than the cross-entropy baseline, with a $p$-value of $5.1\e{-6}$. This loss function was discovered in generation 45, requiring 12,600 2,000-step-equivalent partial evaluations. That is, evolution with 20,000-step full evaluations is over 28-times less sample efficient than evolution with 2,000-step partial evaluations.

These results thus suggest that there is an optimal way to evaluate candidates during evolution, resulting in lower computational cost and better loss functions. Notably, the best evolved loss functions from all three runs (i.e., 200-, 2,000-, and 20,000-step) have similar shapes, reinforcing the idea that partial-evaluations can provide useful performance estimates.

\section{Learning rate sensitivity}
\label{sec:lr_sensitivity}

Loss functions can embody different learning rates implicitly. This section shows that TaylorGLO loss functions' benefits come from more than just metalearning such learning rates. Increases in performance that result from altering the base learning rate with  cross-entropy loss are significantly smaller than those that TaylorGLO provides.

\begin{figure}
  \centering
  \includegraphics[width=0.8\linewidth]{images/allcnnc_lr_sweep.pdf}
  \caption{Effect of varying learning rates in AllCNN-C when trained with the cross-entropy loss on CIFAR-10. For each learning rate, ten models were trained, with up to ten retries if training failed. The majority of training attempts failed for learning rates larger than 0.01. The 0.01 learning rate used in the experiments in this paper results in best stable performance. Overall, the small performance differences that can result from adjusting the learning rate, regardless of stability, are much smaller than those that result from training with TaylorGLO. Thus, TaylorGLO provides a mechanism for improvement beyond implicit adjustments of the learning rate.}
  \label{fig:allcnnc_lr_sweep}
\end{figure}

More specifically, Figure~\ref{fig:allcnnc_lr_sweep} quantifies the effect of varying learning rates on the final testing accuracy of AllCNN-C models trained on CIFAR-10. AllCNN-C was chosen for this analysis since it exhibits the largest variations in performance, making this effect more clear. While learning rates larger than 0.01 (the standard learning rate for AllCNN-C) reach slightly higher accuracies, this effect comes at the cost of less stable training. The majority of models trained with these higher learning rates failed to train. Thus, the standard choice of learning rate for AllCNN-C is appropriate for the cross-entropy loss, and TaylorGLO loss functions are able to improve upon it.

\section{Taylor approximations of the cross-entropy loss }
\label{sec:ce_taylors}

While TaylorGLO's performance originates primarily from discovering better loss functions, it is informative to analyze what role the accuracy of the Taylor approximation plays in it. One way to characterize this effect is to analyze the performance of various Taylor approximations of the cross-entropy loss.

\begin{table}
  \caption{Performance of Taylor approximations of the cross-entropy loss function on AllCNN-C with CIFAR-10. Approximations of different orders, with $\vec{a}=\langle 0.5,0.5 \rangle$, are presented. Presented accuracies are the mean from ten runs. The baseline is the standard cross-entropy loss. Higher-order approximations are better, suggesting a potential (although computationally expensive) opportunity for improvement in the future.} %MNIST experiments ran for 100 generations, while CIFAR-10 experiments ran for 50.
  \vspace{1em}
  \label{tab:ce_approx_results}
  \centering
  {
%   \footnotesize
  \begin{tabular}{lc}
    \toprule
    Loss Function & Mean Accuracy (stddev)\\
    \midrule
    $k=2$ &	0.1034 (0.0101) \\
    $k=3$ &	0.8451 (0.0043) \\
    $k=4$ &	0.8592 (0.0032) \\
    $k=5$ &	0.8649 (0.0042) \\
    Cross-Entropy &	\textbf{0.8965 (0.0021)} \\
 \bottomrule
\end{tabular}
}
\end{table}

Table~\ref{tab:ce_approx_results} provides results from such a study. Bivariate approximations to the cross-entropy loss, centered at $\vec{a}=\langle 0.5,0.5 \rangle$, with different orders $k$ were used to train AllCNN-C models on CIFAR-10. Third-order approximations and above are trainable. Approximations' performance is within a few percentage points of the cross-entropy loss, with higher-order approximations yielding progressively better accuracies, as expected.

The results thus show that third-order TaylorGLO loss functions cannot represent the cross-entropy baseline loss accurately. One possibility for improving TaylorGLO is thus to utilize higher order approximations. However, it is remarkable that TaylorGLO can still find loss functions that outperform the cross-entropy loss. Also, the increase in the number of parameters---and the corresponding increase in computational requirements---may in practice outweigh the benefits from a finer-grained representation. This effect was seen in preliminary experiments, and the third-order approximations (used in this paper) deemed to strike a good balance.

% \begin{figure}
%   \centering
%   \includegraphics[width=0.5\linewidth]{ICLR21 TaylorGLO/images/crossentropy_taylors.pdf}
%   \caption{Performance of Taylor approximations of the cross-entropy loss function. Approximations of different orders, with $\vec{a}=\langle 0.5,0.5 \rangle$, are presented. The baseline is the standard cross-entropy loss.}
%   \label{fig:allcnnc_lr_sweep}
% \end{figure}

% The following approximations, with , were used:

% \begin{equation}
% \frac{1}{2} ((y-0.5) (2 (y-0.5)-2 (x-0.5))-2 (x-0.5) (y-0.5))+0.693147 (x-0.5)- (y-0.5)+0.346574
% \end{equation}

\section{TaylorGLO experiment durations and environmental impact}
\label{sec:comp_costs}

% The cluster where experiments were run had equal numbers of machines in two separate configurations:
% \begin{description}
% 	\item[Configuration 1:] Servers with two 16-core Intel Xeon E5-2683 v4 processors running at a base frequency of 2.1GHz, 264GB of memory, and eight NVIDIA GeForce RTX 1080 Ti GPUs.
% 	\item[Configuration 2:] Servers with two 16-core Intel Xeon Silver 4216 processors running at a base frequency of 2.1GHz, 384GB of memory, and nine NVIDIA GeForce RTX 2080 Ti GPUs.
% \end{description}
The infrastructure that ran the experiments in this paper is located in California, which is estimated to have had an estimated carbon dioxide equivalent total output emission rate of 226.21 kgCO$_2$eq/kWh in 2018 \citep{epa_egrid2018}. This quantity can be used to calculate the climate impact of compute-intensive experiments.

\begin{table}
  \caption{Estimated TaylorGLO experiment durations and total emissions. The estimates assume populations of 20 concurrent candidates and 50 generation runs. Emission values are upper bounds reported in equivalent kilograms of carbon dioxide, thus accounting for other gases of interest. Overall, experiments are short enough that they can each be run over a few days.}
  \vspace{1em}
  \label{tab:carbon_impact}
  \centering
  {
  \footnotesize
  \begin{tabular}{lcc}
    \toprule
    TaylorGLO Experiment & Duration (hours) & Total Emissions (kgCO$_2$eq)\\
    \midrule
	AlexNet on CIFAR-10 & 3.60 & 4.07 \\
    ResNet-20 on CIFAR-10& 10.24 & 11.58 \\
    Pre ResNet-20 on CIFAR-10& 9.26 & 10.48 \\
    AllCNN-C on CIFAR-10& 17.06 & 19.30 \\
    % AllCNN-C + Aux. Classifiers on CIFAR-10& 19.62 & 22.20 \\
    PyramidNet 110a48 on CIFAR-10& 73.86 & 83.53 \\
    Wide ResNet 28-5 on CIFAR-10& 42.90 & 48.52 \\
	Wide ResNet 16-8 on CIFAR-10& 36.08 & 40.80 \\
	Wide ResNet 28-10 on CIFAR-10& 105.30 & 119.10 \\
 \bottomrule
\end{tabular}
}
\end{table}

Table~\ref{tab:carbon_impact} provides estimates of durations and total emissions for various TaylorGLO experiments. Emissions were calculated using the Machine Learning Impact calculator \citep{lacoste2019quantifying}, assuming that no candidates failed evaluation (which would result in slightly lower estimates). Presented values can thus be thought of as being an upper bound. % that experiments were evenly distributed across both hardware configurations specified above, and

Overall, experiment durations are short enough that TaylorGLO can be practically applied to different tasks to find customized loss functions.
